# Supplementary material for: Universal Aspects of High-Temperature Relaxation Dynamics in Random Spin Models
Source: arXiv:2305.02359 source file (2024-06-21)
Supplement: Supplementary file 1 [file supp.pdf]

# Supplementary Material: Universal Aspect of Relaxation Dynamics in Random Spin Models

Tian-Gang Zhou,<sup>1</sup> Wei Zheng,<sup>2,3</sup> and Pengfei Zhang<sup>4,\*</sup>

<sup>1</sup>*Institute for Advanced Study, Tsinghua University, Beijing, 100084, China*

<sup>2</sup>*Hefei National Laboratory for Physical Sciences at the Microscale and Department of Modern Physics, University of Science and Technology of China, Hefei 230026, China*

<sup>3</sup>*CAS Center for Excellence in Quantum Information and Quantum Physics, University of Science and Technology of China, Hefei 230026, China*

<sup>4</sup>*Department of Physics, Fudan University, Shanghai, 200438, China*

(Dated: May 2, 2023)

In this Supplementary Material, we present: (1) The formulation of the equilibrium Green's function; (2) The symmetry of the Green's function; (3) Details of the numerical simulation; (4) Explicit calculation of the self energy; (5) Derivation of the normal mode equation with regular interactions; (6) Derivation of the normal mode equation with Brownian interactions; (7) Susceptibility in thermal equilibrium.

## I. THE FORMULATION OF THE EQUILIBRIUM GREEN'S FUNCTION

To further proceed, we need the real-time approach. We begin with the greater and lesser Green's functions in real-time defined as

$$\begin{aligned} G_{ss'}^>(t_1, t_2) &\equiv -i \frac{1}{N} \sum_l \left\langle c_{l,s}(t_1) c_{l,s'}^\dagger(t_2) \right\rangle, \\ G_{ss'}^<(t_1, t_2) &\equiv i \frac{1}{N} \sum_l \left\langle c_{l,s'}^\dagger(t_2) c_{l,s}(t_1) \right\rangle, \end{aligned} \quad (1)$$

as well as the retarded and advanced Green's function defined as

$$G_{ss'}^{R/A}(t_1, t_2) \equiv \mp i \Theta(\pm t_{12}) \frac{1}{N} \sum_l \left\langle \{c_{l,s}(t_1), c_{l,s'}^\dagger(t_2)\} \right\rangle, \quad (2)$$

where  $\Theta(t)$  is the Heaviside step function and we have defined  $t_{12} = t_1 - t_2$ . In the thermal equilibrium, all Green's functions are only functions of  $t_{12}$  due to the time-translational symmetry. To solve the real-time Green's functions self-consistently, we introduce the spectral function as

$$G^R(\omega) = \int dz \frac{\rho(z)}{z - \omega + i0}, \quad (3)$$

which implies  $\rho(\omega) = -\text{Im}G^R(\omega)/\pi$ . Other Green's functions are determined by the fluctuation-dissipation theorem as

$$\begin{aligned} G^<(\omega) &= 2\pi i n_F(\omega) \rho(\omega), \\ G^>(\omega) &= -2\pi i n_F(-\omega) \rho(\omega), \end{aligned} \quad (4)$$

where  $n_F(\omega)$  is the Fermi-Dirac distribution function. For later convenience, we introduce the Keldysh Green's function

$$\begin{aligned} G^K(\omega) &\equiv G^>(\omega) + G^<(\omega) \\ &= (2n_F(\omega) - 1) 2\pi \rho(\omega) \\ &= (1 - 2n_F(\omega)) (G^R(\omega) - G^A(\omega)) \end{aligned} \quad (5)$$

---

\* PengfeiZhang.physics@gmail.com

To derive the self-consistent equation for the spectral function, we the Schwinger-Dyson equation in real time reads

$$G^R(\omega)^{-1} = \omega + \frac{\hbar}{2}\sigma^x - \Sigma^R(\omega) \quad (6)$$

, with real-time self-energies obtained via large- $N$  and the melon diagram approximations are given by

$$\begin{aligned} \Sigma^{\geq}(t_1, t_2) &= \frac{J^2}{4} \sum_{\alpha, \alpha'} \xi_{\alpha} \xi_{\alpha'} \\ \sigma^{\alpha'} G^{\geq}(t_1, t_2) \sigma^{\alpha} \text{Tr} \left[ \sigma^{\alpha'} G^{\geq}(t_1, t_2) \sigma^{\alpha} G^{\leq}(t_2, t_1) \right], \end{aligned} \quad (7)$$

Here  $\Sigma^{\geq}, \sigma^{\alpha}$  and  $G^{\geq}$  are all  $2 \times 2$  matrix corresponding to spin indexes, and trace operation is applied on the spin indexes. Furthermore,  $\Sigma^{R/A}$  and  $\Sigma^K$  related to  $\Sigma^{\geq}$  as

$$\begin{aligned} \Sigma^{R/A}(t_1, t_2) &= \pm \Theta(\pm t_{12}) (\Sigma^{>}(t_1, t_2) - \Sigma^{<}(t_1, t_2)), \\ \Sigma^K(t_1, t_2) &= (\Sigma^{>}(t_1, t_2) + \Sigma^{<}(t_1, t_2)). \end{aligned} \quad (8)$$

Iteratively solving Eq. (6) gives the spectral function  $\rho_{ss'}(\omega)(s, s' = \uparrow, \downarrow)$  and real-time Green's functions.

In numerics, we choose the discretization of time domain  $t$  and frequency domain  $\omega$  to be 3001. The cutoff in time domain is  $[-\Lambda_t, \Lambda_t] = [-20.0, 20.0]$ , and frequency domain is time domain is  $[-\Lambda_{\omega}, \Lambda_{\omega}] = [-12.0, 12.0]$ .

## II. THE SYMMETRY OF THE GREEN'S FUNCTION

In this section, we analyze the symmetries of the fermion Green's function encoded in random spin model

$$\hat{H}(t) = \sum_{1 \leq i < j \leq N} J_{ij} (\hat{S}_i^x \hat{S}_j^x + \xi_2 \hat{S}_i^y \hat{S}_j^y + \xi_3 \hat{S}_i^z \hat{S}_j^z) - h(t) \sum_{1 \leq i \leq N} \hat{S}_i^x. \quad (9)$$

There are two symmetries crucial for the later simplification. The first can be regarded as  $\pi$  rotation of axis  $x$ .

$$\begin{aligned} \hat{c}_{s_1} &\rightarrow \sum_{s'} (i\sigma^x)_{s_1 s'} \hat{c}_{s'} \\ \hat{c}_{s_1}^{\dagger} &\rightarrow \sum_{s'} \hat{c}_{s'}^{\dagger} (-i\sigma^x)_{s' s_1}. \end{aligned} \quad (10)$$

With symmetry in Eq. (10),  $\{\hat{S}^x, \hat{S}^y, \hat{S}^z\}$  is mapped to  $\{\hat{S}^x, -\hat{S}^y, -\hat{S}^z\}$ , and therefore keeps Eq. (9) invariant. As a consequence, the symmetry of Green's function leads to

$$\begin{aligned} G_{s_1 s_2}^{>}(t_1, t_2) &= -i \langle \hat{c}_{s_1}(t_1) \hat{c}_{s_2}^{\dagger}(t_2) \rangle \\ &= \sum_{s' s''} \sigma_{s_1 s'}^x G_{s' s''}^{>}(t_1, t_2) \sigma_{s'' s_2}^x \\ &= \begin{pmatrix} G_{\downarrow\downarrow}^{>}(t_1, t_2) & G_{\downarrow\uparrow}^{>}(t_1, t_2) \\ G_{\uparrow\downarrow}^{>}(t_1, t_2) & G_{\uparrow\uparrow}^{>}(t_1, t_2) \end{pmatrix}_{s_1 s_2} \end{aligned} \quad (11)$$

The second symmetry is combined with particle-hole symmetry and rotation, which reads as

$$\begin{aligned} \hat{c}_{s_1} &\rightarrow \sum_{s'} (i\sigma^y)_{s_1 s'} \hat{c}_{s'}^{\dagger} \\ \hat{c}_{s_1}^{\dagger} &\rightarrow \sum_{s'} \hat{c}_{s'} (-i\sigma^y)_{s' s_1}. \end{aligned} \quad (12)$$

Similarly, with symmetry in Eq. (12),  $\{\hat{S}^x, \hat{S}^y, \hat{S}^z\}$  is mapped to  $\{\hat{S}^x, -\hat{S}^y, \hat{S}^z\}$ , and therefore keeps Eq. (9) invariant. Also, the symmetry of Green's function leads to

$$\begin{aligned} G_{s_1 s_2}^{>}(t_1, t_2) &= -i \langle \hat{c}_{s_1}(t_1) \hat{c}_{s_2}^{\dagger}(t_2) \rangle \\ &= - \sum_{s' s''} \sigma_{s_1 s'}^y G_{s'' s'}^{<}(t_2, t_1) \sigma_{s'' s_2}^y \\ &= \begin{pmatrix} -G_{\uparrow\uparrow}^{<}(t_2, t_1) & G_{\uparrow\downarrow}^{<}(t_2, t_1) \\ G_{\downarrow\uparrow}^{<}(t_2, t_1) & -G_{\downarrow\downarrow}^{<}(t_2, t_1) \end{pmatrix}_{s_1 s_2}, \end{aligned} \quad (13)$$

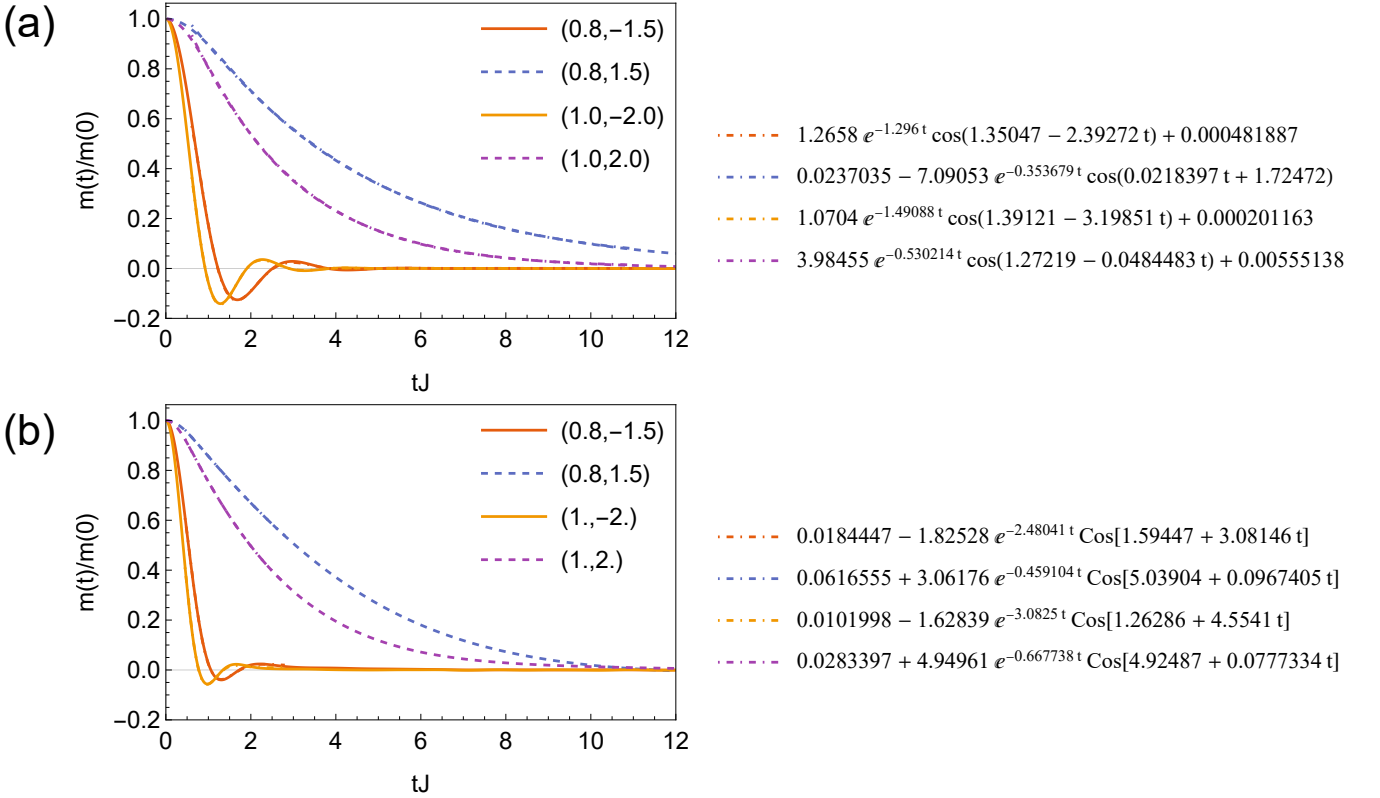

FIG. 1. Fitting of (a) the large- $N$  dynamics; (b) the exact diagonalization dynamics corresponding to the main text fig. (2).

where the second line to the third line uses the symmetry obtained in Eq. (11). Finally, we can exchange  $>$  and  $<$  symbols in Eq. (11) and Eq. (11) to obtain another two symmetry in terms of Green's function.

### III. DETAILS OF THE NUMERICAL SIMULATION

#### A. Kadanoff-Baym equation

We choose the discretiation of Green's function matrix  $G^{\geq}(t_1, t_2)$  to be  $4001 \times 4001$ , with a cutoff  $t_1, t_2 \in [-\Lambda_t, \Lambda_t] = [-20.0, 20.0]$ . As we discussed in the main text, for  $t_1, t_2 < 0$ , the system is prepared in thermal equilibrium with  $G^{\geq}(t_1, t_2) = G_{\beta}^{\geq}(t_{12})$ .

To obtain the oscillation frequency, we fit the magnetization dynamics with the formula

$$m(t) = m_0 \cos(\Omega t + \theta) e^{-\Gamma t} + m_{\text{offset}}. \quad (14)$$

Here  $m_0$  is the amplitude,  $\theta$  is the phase,  $\Gamma$  is the quasi-particle decay rate, and  $m_{\text{offset}}$  is the offset which is significant in the finite  $N$  exact diagonalization numerics.

We observe that the offset  $m_{\text{offset}}$  is negligibly small in the order of  $10^{-3}$  when the fitting region covers enough long time, which is consistent with the symmetry reason. Therefore, we choose fitting region  $tJ \in [0.61, 11]$  in fig. 1(a) to ensure the correctness of fitting. We have also checked that the fitting parameters are not sensitive to the detailed fitting region if it covers enough early time and long time regions. In numerics, we use Mathematica `NonlinearModelFit` function to perform the non-linear fitting.

#### B. Exact Diagonalization

Due to the finite  $N$  correction, we find the result deviates from the formula Eq. (14) if fitting includes the entire long-time and early-time region. Therefore, we aim to focus on the small  $m(t)/m(0)$  region where oscillations happen.

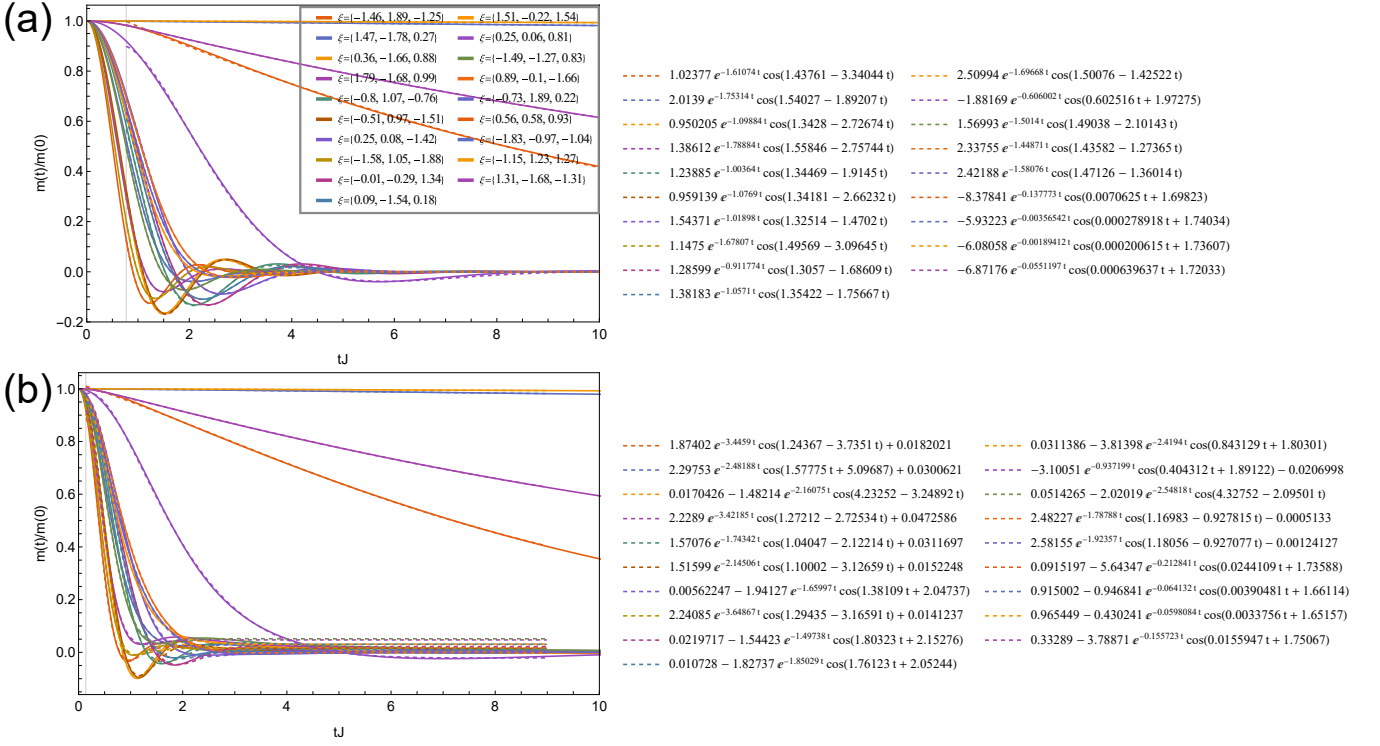

FIG. 2. Fitting of (a) the large- $N$  dynamics; (b) the exact diagonalization dynamics corresponding to the main text fig. (3). The solid line is the numerical data, and the dashed line is the fitting curve. The inset legend lists each anisotropic parameter corresponding to the 19 cases in the main text. Besides, the right panel shows the fitting functions for each case.

Here we take fitting region  $tJ \in [0.45, 2.8]$ . From fig. 1(b) we find the fitting precisely matches with the dynamics data. Although the oscillation frequency is more sensitive to the fitting region compared with the large- $N$  case, the behavior of oscillation frequency in terms of anisotropic parameter qualitatively remains no change.

### C. Estimation of frequency and error bar

Fig. (3) in the main text shows the estimation of frequency and error bars with random anisotropic parameters. Here we show the detailed fitting result in fig. 2, where the initial temperature and external magnetic field is  $\beta J = 0.04$ ,  $\bar{J} = 0$  and  $h/J = 10$ .

The choice of the fitting region is naturally uncertain. First, the theoretical prediction of the oscillation frequency acquires the assumption of small  $m(t)$ , but the small  $m(t)$  time region is not uniquely defined. Secondly, especially for ED numerics, finite system size leads to untrustable results in the late time limit. Therefore it is reasonable only to consider the early time when fitting the ED numerics, which also introduces uncertainty of fitting region.

The error bars of the fitting frequency arise from such uncertainty. To quantifies such error, we separately consider two different numerical approaches.

- For the large- $N$  data, we choose the time region begins at different values:  $t_{\text{begin}}J = 0, 0.05, 0.1, \dots, 1.2$ , and ends at the same point  $t_{\text{end}}J = 10.0$ . We fit these frequencies and take the standard deviation as the error bars.
- For the ED data, we choose the time region begins at different values:  $t_{\text{begin}}J = 0, 0.08, 0.16, \dots, 0.4$ , and ends at also different points  $t_{\text{end}}J = 3.0, 4.0, \dots, 9.0$ . We take a combination of these beginning and ending points and take the standard deviation among these frequencies as the error bars.

We summarize the detailed fitting region in table. I. Notice that for the ED approach, we need a larger ending fitting time for the small frequency cases, but in other cases, we choose a smaller ending fitting time to avoid the finite  $N$  effect.

| Cases                         | 1     | 2     | 3     | 4     | 5     | 6     | 7     | 8     | 9     | 10    | 11    | 12   | 13    | 14    | 15    | 16   | 17    | 18    | 19    |
|-------------------------------|-------|-------|-------|-------|-------|-------|-------|-------|-------|-------|-------|------|-------|-------|-------|------|-------|-------|-------|
| $\xi_1$                       | -1.46 | 1.47  | 0.36  | 1.79  | -0.8  | -0.51 | 0.25  | -1.58 | -0.01 | 0.09  | 1.51  | 0.25 | -1.49 | 0.89  | -0.73 | 0.56 | -1.83 | -1.15 | 1.31  |
| $\xi_2$                       | 1.89  | -1.78 | -1.66 | -1.68 | 1.07  | 0.97  | 0.08  | 1.05  | -0.29 | -1.54 | -0.22 | 0.06 | -1.27 | -0.1  | 1.89  | 0.58 | -0.97 | 1.23  | -1.68 |
| $\xi_3$                       | -1.25 | 0.27  | 0.88  | 0.99  | -0.76 | -1.51 | -1.42 | -1.88 | 1.34  | 0.18  | 1.54  | 0.81 | 0.83  | -1.66 | 0.22  | 0.93 | -1.04 | 1.27  | -1.31 |
| $\Omega_{\text{KB}}$          | 3.34  | 1.89  | 2.73  | 2.76  | 1.91  | 2.66  | 1.47  | 3.10  | 1.69  | 1.76  | 1.43  | 0.60 | 2.10  | 1.27  | 1.36  | 0.01 | 0.00  | 0.00  | 0.00  |
| $\sigma_{\Omega_{\text{KB}}}$ | 0.19  | 0.17  | 0.13  | 0.20  | 0.12  | 0.13  | 0.10  | 0.20  | 0.10  | 0.12  | 0.12  | 0.03 | 0.16  | 0.10  | 0.11  | 0.01 | 0.00  | 0.00  | 0.01  |
| $\Omega_{\text{ED}}$          | 3.74  | 1.58  | 3.25  | 2.73  | 2.12  | 3.13  | 1.38  | 3.17  | 1.80  | 1.76  | 0.84  | 0.40 | 2.10  | 0.93  | 0.93  | 0.02 | 0.00  | 0.00  | 0.02  |
| $\sigma_{\Omega_{\text{ED}}}$ | 0.59  | 0.46  | 0.31  | 0.52  | 0.17  | 0.30  | 0.05  | 0.49  | 0.11  | 0.10  | 0.33  | 0.16 | 0.23  | 0.08  | 0.16  | 0.05 | 0.04  | 0.04  | 0.04  |
| $\Omega_{\text{Th}}$          | 3.53  | 1.73  | 3.04  | 2.69  | 2.08  | 2.97  | 1.55  | 3.17  | 1.85  | 1.87  | 1.22  | 0.63 | 2.07  | 1.14  | 1.19  | 0.00 | 0.00  | 0.00  | 0.00  |
| $t_{\text{begin,KB}}J$        | 0.75  | 0.75  | 0.75  | 0.75  | 0.75  | 0.75  | 0.75  | 0.75  | 0.75  | 0.75  | 0.75  | 0.75 | 0.75  | 0.75  | 0.75  | 0.75 | 0.75  | 0.75  | 0.75  |
| $t_{\text{end,KB}}J$          | 10    | 10    | 10    | 10    | 10    | 10    | 10    | 10    | 10    | 10    | 10    | 10   | 10    | 10    | 10    | 10   | 10    | 10    | 10    |
| $t_{\text{begin,ED}}J$        | 0.15  | 0.15  | 0.15  | 0.15  | 0.15  | 0.15  | 0.15  | 0.15  | 0.15  | 0.15  | 0.15  | 0.15 | 0.15  | 0.15  | 0.15  | 0.15 | 0.15  | 0.15  | 0.15  |
| $t_{\text{end,ED}}J$          | 3.5   | 3.5   | 3.5   | 3.5   | 3.5   | 3.5   | 3.5   | 3.5   | 3.5   | 3.5   | 3.5   | 9    | 3.5   | 9     | 9     | 9    | 9     | 9     | 9     |

TABLE I. The detailed parameters and result for each case.  $(\xi_1, \xi_2, \xi_3)$  means anisotropic parameters.  $\Omega_{\text{KB}}, \Omega_{\text{ED}}, \Omega_{\text{Th}}$  are the fitting frequencies from Kadanoff-Baym numerics, ED numerics, and theoretical prediction.  $\sigma_{\Omega_{\text{KB}}}, \sigma_{\Omega_{\text{ED}}}$  are the standard deviations for KB and ED numerics.  $[t_{\text{begin,KB}}J, t_{\text{end,KB}}J]$  and  $[t_{\text{begin,ED}}J, t_{\text{end,ED}}J]$  are the fit region which lead to the  $\Omega_{\text{KB}}, \Omega_{\text{ED}}$  numerics data of the main text fig. 3.

#### IV. EXPLICIT CALCULATION OF THE SELF-ENERGY

Starting from Eq. (7), we derivate the corresponding analytical formula. We first consider the trace part

$\text{Tr} [\sigma^{\alpha'} G^{\geq}(t_1, t_2) \sigma^{\alpha} G^{\leq}(t_2, t_1)]$ . In the basis of  $\alpha', \alpha = \{x, y, z\}$ , trace part becomes

$$\begin{aligned}
& \text{Tr} [\sigma^{\alpha'} G^{\geq}(t_1, t_2) \sigma^{\alpha} G^{\leq}(t_2, t_1)] \\
&= -\text{Tr} [\sigma^y \sigma^{\alpha'} G^{\geq}(t_1, t_2) \sigma^{\alpha} \sigma^y G^{\geq}(t_1, t_2)] \\
&= \begin{pmatrix} -2G_{\uparrow\uparrow}^{\geq}(t_1, t_2)^2 + 2G_{\uparrow\downarrow}^{\geq}(t_1, t_2)^2 & 0 & 0 \\ 0 & -2G_{\uparrow\uparrow}^{\geq}(t_1, t_2)^2 - 2G_{\uparrow\downarrow}^{\geq}(t_1, t_2)^2 & 4iG_{\uparrow\uparrow}^{\geq}(t_1, t_2)G_{\uparrow\downarrow}^{\geq}(t_1, t_2) \\ 0 & -4iG_{\uparrow\uparrow}^{\geq}(t_1, t_2)G_{\uparrow\downarrow}^{\geq}(t_1, t_2) & -2G_{\uparrow\uparrow}^{\geq}(t_1, t_2)^2 - 2G_{\uparrow\downarrow}^{\geq}(t_1, t_2)^2 \end{pmatrix}_{\alpha'\alpha}. \quad (15)
\end{aligned}$$

The second line applies the symmetry Eq. (13) and implicitly use Eq. (11) to ensure  $(G^{\geq})^T = G^{\leq}$ . The disappearance of off-diagonal certain matrix elements is non-trivial. For example, we take  $\alpha' = x, \alpha = z$ .

$$\begin{aligned}
& -\text{Tr} [\sigma^y \sigma^x G^{\geq}(t_1, t_2) \sigma^z \sigma^y G^{\geq}(t_1, t_2)] \\
&= -\text{Tr} [\sigma^y G^{\geq}(t_1, t_2) \sigma^x \sigma^z \sigma^y G^{\geq}(t_1, t_2)] \\
&= i\text{Tr} [\sigma^y G^{\geq}(t_1, t_2) G^{\geq}(t_1, t_2)] \\
&= i\text{Tr} \left[ \sigma^y \begin{pmatrix} G_{\uparrow\uparrow}^{\geq}(t_1, t_2)^2 + G_{\uparrow\downarrow}^{\geq}(t_1, t_2)^2 & 2G_{\uparrow\uparrow}^{\geq}(t_1, t_2)G_{\uparrow\downarrow}^{\geq}(t_1, t_2) \\ 2G_{\uparrow\uparrow}^{\geq}(t_1, t_2)G_{\uparrow\downarrow}^{\geq}(t_1, t_2) & G_{\uparrow\uparrow}^{\geq}(t_1, t_2)^2 + G_{\uparrow\downarrow}^{\geq}(t_1, t_2)^2 \end{pmatrix} \right].
\end{aligned}$$

Since the non-zero elements in Pauli matrix  $\sigma^y$  are  $\pm i$  separately, we find  $\text{Tr} [\sigma^y G^{\geq}(t_1, t_2) G^{\geq}(t_1, t_2)] = 0$ . Similarly, the  $\alpha' = x, \alpha = y$  case corresponds to  $\text{Tr} [\sigma^z G^{\geq}(t_1, t_2) G^{\geq}(t_1, t_2)] = 0$  and therefore the trace part vanishes.

However, it is special for  $\alpha' = y, \alpha = z$ , which reduced to the final result  $\text{Tr} [\sigma^x G^{\geq}(t_1, t_2) G^{\geq}(t_1, t_2)] \neq 0$ , since  $\sigma^x$  only contains two 1 elements. Hence, the only non-zero off-diagonal trace part is  $\alpha' = y, \alpha = z$ , and  $\alpha' = z, \alpha = y$ .

To further calculate the self-energy, we show each non-zero contribution in Eq. (7).

a.  $\alpha' = x, \alpha = x$

$$\frac{1}{2} J^2 \xi_1^2 \begin{pmatrix} G_{\uparrow\uparrow}^{\geq}(t_1, t_2) & G_{\uparrow\downarrow}^{\geq}(t_1, t_2) \\ G_{\uparrow\downarrow}^{\geq}(t_1, t_2) & G_{\uparrow\uparrow}^{\geq}(t_1, t_2) \end{pmatrix} \begin{pmatrix} -G_{\uparrow\uparrow}^{\geq}(t_1, t_2)^2 + G_{\uparrow\downarrow}^{\geq}(t_1, t_2)^2 \end{pmatrix} \quad (16)$$

b.  $\alpha' = y, \alpha = y$

$$\frac{1}{2} J^2 \xi_2^2 \begin{pmatrix} -G_{\uparrow\uparrow}^{\geq}(t_1, t_2) & G_{\uparrow\downarrow}^{\geq}(t_1, t_2) \\ G_{\uparrow\downarrow}^{\geq}(t_1, t_2) & -G_{\uparrow\uparrow}^{\geq}(t_1, t_2) \end{pmatrix} \begin{pmatrix} G_{\uparrow\uparrow}^{\geq}(t_1, t_2)^2 + G_{\uparrow\downarrow}^{\geq}(t_1, t_2)^2 \end{pmatrix} \quad (17)$$

c.  $\alpha' = z, \alpha = z$

$$\frac{1}{2}J^2\xi_3^2 \begin{pmatrix} -G_{\uparrow\uparrow}^{\geq}(t_1, t_2) & G_{\uparrow\downarrow}^{\geq}(t_1, t_2) \\ G_{\uparrow\downarrow}^{\geq}(t_1, t_2) & -G_{\uparrow\uparrow}^{\geq}(t_1, t_2) \end{pmatrix} \left( G_{\uparrow\uparrow}^{\geq}(t_1, t_2)^2 + G_{\uparrow\downarrow}^{\geq}(t_1, t_2)^2 \right) \quad (18)$$

d.  $\alpha' = y, \alpha = z$

$$J^2\xi_2\xi_3 \begin{pmatrix} G_{\uparrow\downarrow}^{\geq}(t_1, t_2) & -G_{\uparrow\uparrow}^{\geq}(t_1, t_2) \\ -G_{\uparrow\uparrow}^{\geq}(t_1, t_2) & G_{\uparrow\downarrow}^{\geq}(t_1, t_2) \end{pmatrix} \left( G_{\uparrow\uparrow}^{\geq}(t_1, t_2)G_{\uparrow\downarrow}^{\geq}(t_1, t_2) \right) \quad (19)$$

e.  $\alpha' = z, \alpha = y$

$$J^2\xi_2\xi_3 \begin{pmatrix} G_{\uparrow\downarrow}^{\geq}(t_1, t_2) & -G_{\uparrow\uparrow}^{\geq}(t_1, t_2) \\ -G_{\uparrow\uparrow}^{\geq}(t_1, t_2) & G_{\uparrow\downarrow}^{\geq}(t_1, t_2) \end{pmatrix} \left( G_{\uparrow\uparrow}^{\geq}(t_1, t_2)G_{\uparrow\downarrow}^{\geq}(t_1, t_2) \right) \quad (20)$$

Finally, we arrive the full self-energy

$$\Sigma^{\geq}(t_1, t_2) = \frac{1}{2}J^2 \begin{pmatrix} -\xi^2 G_{\uparrow\uparrow}^{\geq}(t_1, t_2)^3 + AG_{\uparrow\uparrow}^{\geq}(t_1, t_2)G_{\uparrow\uparrow}^{\geq}(t_1, t_2)^2 & AG_{\uparrow\uparrow}^{\geq}(t_1, t_2)^2 G_{\uparrow\downarrow}^{\geq}(t_1, t_2) + \xi^2 G_{\uparrow\downarrow}^{\geq}(t_1, t_2)^3 \\ AG_{\uparrow\uparrow}^{\geq}(t_1, t_2)^2 G_{\uparrow\downarrow}^{\geq}(t_1, t_2) + \xi^2 G_{\uparrow\downarrow}^{\geq}(t_1, t_2)^3 & -\xi^2 G_{\uparrow\uparrow}^{\geq}(t_1, t_2)^3 + AG_{\uparrow\uparrow}^{\geq}(t_1, t_2)G_{\uparrow\downarrow}^{\geq}(t_1, t_2)^2 \end{pmatrix}, \quad (21)$$

where the polynomials  $\xi^2 = \xi_1^2 + \xi_2^2 + \xi_3^2$  and  $A = -\xi_1^2 + \xi_2^2 - 4\xi_2\xi_3 + \xi_3^2$ .

## V. DERIVATION OF THE NORMAL MODE EQUATION WITH REGULAR INTERACTIONS

### A. Derivation of Eq. (6) in the main text

As formulated in the main text, the perturbation is applied on  $(G^a)_{ss'} = (G^{a, \beta_f})_{ss'} + \delta G_{\uparrow\downarrow}^a (\delta_{s\uparrow}\delta_{s'\downarrow} + \delta_{s'\uparrow}\delta_{s\downarrow})$ , with causality index  $a = \geq$ , and the perturbation assumption  $\delta G_{\uparrow\downarrow}^a \ll G_{ss}^a$  where  $s = \uparrow, \downarrow$ .

According to the Lorentzian approximation

$$G_{\uparrow\uparrow}^{R/A, \beta_f}(t) \approx \mp i\Theta(\pm t)e^{-\Gamma|t|/2}, \quad G_{\uparrow\uparrow}^{\geq, \beta_f}(t) \approx \mp ie^{-\Gamma|t|/2}/2. \quad (22)$$

We have  $G^{K, \beta_f} = G^{>, \beta_f} + G^{<, \beta_f} \approx 0$ . Furthermore, we can assume  $\delta G_{\uparrow\downarrow}^{\geq} = \frac{1}{2}\delta G_{\uparrow\downarrow}^K$ , which is consistent with the definition of Keldysh Green's function in Eq. (5).

We consider the self-consistent condition

$$G^K = G^R \circ \Sigma^K \circ G^A. \quad (23)$$

The perturbation in the off-diagonal element reads as

$$G_{\uparrow\downarrow}^K = \sum_{ss'=\uparrow, \downarrow} G_{\uparrow s}^R \circ \Sigma_{ss'}^K \circ G_{s'\downarrow}^A. \quad (24)$$

We discuss the result separately

a.  $s = \uparrow, s' = \uparrow$

$$\begin{aligned} \Sigma_{\uparrow\uparrow}^K &= \Sigma_{\uparrow\uparrow}^> + \Sigma_{\uparrow\uparrow}^< \\ &= \frac{1}{2}J^2A \left( G_{\uparrow\uparrow}^>(t_1, t_2)G_{\uparrow\downarrow}^>(t_1, t_2)^2 + G_{\uparrow\uparrow}^<(t_1, t_2)G_{\uparrow\downarrow}^<(t_1, t_2)^2 \right) - \frac{1}{2}J^2\xi^2 \left( G_{\uparrow\uparrow}^>(t_1, t_2)^3 + G_{\uparrow\uparrow}^<(t_1, t_2)^3 \right) \\ &= 0 \left( \delta G_{\uparrow\downarrow}^{\geq} \right)^2 + 0 \end{aligned} \quad (25)$$

The 0 is due to the form of high temperature Green's function Eq. (22), and  $G_{\uparrow\downarrow}^A$  in the Eq. (24) is the first order perturbation. Therefore this term vanishes.

b.  $s = \uparrow, s' = \downarrow$

$$\begin{aligned}
\Sigma_{\uparrow\downarrow}^K &= \Sigma_{\uparrow\downarrow}^> + \Sigma_{\uparrow\downarrow}^< \\
&= \frac{1}{2} J^2 A \left( G_{\uparrow\uparrow}^>(t_1, t_2)^2 G_{\uparrow\downarrow}^>(t_1, t_2) + G_{\uparrow\uparrow}^<(t_1, t_2)^2 G_{\uparrow\downarrow}^<(t_1, t_2) \right) + \frac{1}{2} J^2 \xi^2 \left( G_{\uparrow\downarrow}^>(t_1, t_2)^3 + G_{\uparrow\downarrow}^<(t_1, t_2)^3 \right) \\
&= \frac{1}{2} J^2 A \left( G_{\uparrow\uparrow}^{>, \beta_f}(t_1, t_2)^2 \delta G_{\uparrow\downarrow}^>(t_1, t_2) + G_{\uparrow\uparrow}^{<, \beta_f}(t_1, t_2)^2 \delta G_{\uparrow\downarrow}^<(t_1, t_2) \right) + \frac{1}{2} J^2 \xi^2 \left( \left( \delta G_{\uparrow\downarrow}^>(t_1, t_2) \right)^3 + \left( \delta G_{\uparrow\downarrow}^<(t_1, t_2) \right)^3 \right) \\
&\approx \frac{1}{2} J^2 A \left( G_{\uparrow\uparrow}^{>, \beta_f}(t_1, t_2)^2 \delta G_{\uparrow\downarrow}^>(t_1, t_2) + G_{\uparrow\uparrow}^{<, \beta_f}(t_1, t_2)^2 \delta G_{\uparrow\downarrow}^<(t_1, t_2) \right) \\
&= \frac{1}{4} J^2 A \left( G_{\uparrow\uparrow}^{>, \beta_f}(t_1, t_2)^2 + G_{\uparrow\uparrow}^{<, \beta_f}(t_1, t_2)^2 \right) \delta G_{\uparrow\downarrow}^K(t_1, t_2)
\end{aligned} \tag{26}$$

The approximate equal sign means to keep the first order correction of  $\delta G_{\uparrow\downarrow}^a$  and ignore the high order term. Then we find the zero's order of  $\Sigma_{\uparrow\downarrow}^K$  is zero, and therefore  $\delta \Sigma_{\uparrow\downarrow}^K = \frac{1}{4} J^2 A \left( G_{\uparrow\uparrow}^{>, \beta_f}(t_1, t_2)^2 + G_{\uparrow\uparrow}^{<, \beta_f}(t_1, t_2)^2 \right) \delta G_{\uparrow\downarrow}^K(t_1, t_2)$  leads to the same result in the main text Eq. (6). Also, we notice that in this case  $G_{\uparrow s}^R, G_{s' \downarrow}^A$  are both zero's order, which satisfies the linearized equation  $\delta G_{\uparrow\downarrow}^K = G_{\uparrow\uparrow}^{R, \beta_f} \circ \delta \Sigma_{\uparrow\downarrow}^K \circ G_{\uparrow\uparrow}^{A, \beta_f}$ .

- c.  $s = \downarrow, s' = \uparrow$  Similar to the case (b).  
d.  $s = \downarrow, s' = \downarrow$  Similar to the case (a).

## B. Normal modes

Starting from Eq. (6) in the main text, we apply the Lorentz approximation

$$\begin{aligned}
G_{ss'}^<<(t) &= \pm \frac{i}{2} e^{-\frac{|t|\Gamma}{2}} \delta_{ss'} \\
G_{ss'}^{R/A}(t) &= \pm i e^{\mp \frac{t\Gamma}{2}} \Theta(\pm t) \delta_{ss'} \\
G_{ss'}^K(t) &= G_{ss'}^>(t) + G_{ss'}^<(t) = 0
\end{aligned} \tag{27}$$

It leads to the convolution equation in the time domain

$$\begin{aligned}
e^{-\frac{\lambda}{2}(t_1+t_4)} \varphi(t_{14}) &= G_{\uparrow\uparrow}^R \circ \left( -\frac{1}{8} J^2 A e^{-|t_2-t_3|\Gamma - \frac{\lambda}{2}(t_2+t_3)} \varphi(t_{23}) \right) \circ G_{\downarrow\downarrow}^A \\
&= -\frac{1}{8} J^2 A \int dt_2 dt_3 e^{-\frac{\Gamma}{2}(t_1-t_2)} \Theta(t_1-t_2) e^{-|t_2-t_3|\Gamma - \frac{\lambda}{2}(t_2+t_3)} e^{\frac{\Gamma}{2}(t_3-t_4)} \Theta(-t_3+t_4) \varphi(t_{23}).
\end{aligned} \tag{28}$$

Here  $A = -\xi_1^2 + \xi_2^2 - 4\xi_2\xi_3 + \xi_3^2$  is the polynomial in terms of the anisotropic parameters. Rearrange the variable

$$e^{-\frac{\lambda-\Gamma}{2}(t_1+t_4)} \varphi(t_{14}) = -\frac{1}{8} J^2 A \int dt_2 dt_3 \Theta(t_1-t_2) \Theta(-t_3+t_4) e^{-|t_2-t_3|\Gamma - \frac{\lambda-\Gamma}{2}(t_2+t_3)} \varphi(t_{23}) \tag{29}$$

Apply  $\partial_{t_1}$

$$e^{-\frac{\lambda-\Gamma}{2}(t_1+t_4)} \left[ -\frac{\lambda-\Gamma}{2} \varphi(t_{14}) + \partial_{t_1} \varphi(t_{14}) \right] = -\frac{1}{8} J^2 A \int dt_2 dt_3 \delta(t_1-t_2) \Theta(-t_3+t_4) e^{-|t_2-t_3|\Gamma - \frac{\lambda-\Gamma}{2}(t_2+t_3)} \varphi(t_{23}) \tag{30}$$

Apply  $\partial_{t_4}$

$$\begin{aligned}
e^{-\frac{\lambda-\Gamma}{2}(t_1+t_4)} \left[ \left( \frac{\lambda-\Gamma}{2} \right)^2 \varphi(t_{14}) + \partial_{t_4} \partial_{t_1} \varphi(t_{14}) \right] &= -\frac{1}{8} J^2 A \int dt_2 dt_3 \delta(t_1-t_2) \delta(-t_3+t_4) e^{-|t_2-t_3|\Gamma - \frac{\lambda-\Gamma}{2}(t_2+t_3)} \varphi(t_{23}) \\
&= -\frac{1}{8} J^2 A e^{-|t_1-t_4|\Gamma - \frac{\lambda-\Gamma}{2}(t_1+t_4)} \varphi(t_{14})
\end{aligned} \tag{31}$$

Therefore we finally arrive at the normal mode equations

$$-\frac{(\Gamma-\lambda)^2}{4} \varphi(t_{14}) = -\partial_{t_{14}}^2 \varphi(t_{14}) + \frac{A}{8} J^2 e^{-\Gamma|t_{14}|} \varphi(t_{14}), \tag{32}$$

As discussed in the main text, the positive and negative of  $A$  determine the oscillation and non-oscillation behaviors in the quench dynamics. For clarity, the contour plot of  $A$  is shown in fig. 3.

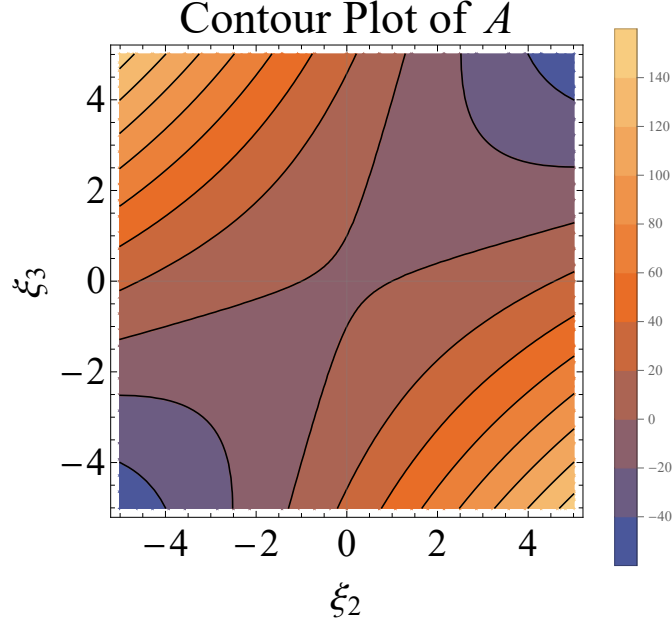

FIG. 3. The contour plot of polynomial  $A$ . The legend shows the  $A > 0$  and  $A < 0$  region.

## VI. DERIVATION OF THE NORMAL MODE EQUATION WITH BROWNIAN INTERACTIONS

To check the effect of coherence, we place  $J_{ij}$  in the Hamiltonian Eq. (9) with Brownian variables  $J_{ij}(t)$ , where  $\overline{J_{ij}(t_1)J_{ij}(t_2)} = 4J^2/N\delta(t_1 - t_2)$ . The self energy is replaced by

$$\Sigma^{\geq}(t_1, t_2) = \frac{1}{2}J^2\delta(t_1 - t_2) \begin{pmatrix} -\xi^2 G_{\uparrow\uparrow}^{\geq}(t_1, t_2)^3 + AG_{\uparrow\uparrow}^{\geq}(t_1, t_2)G_{\uparrow\downarrow}^{\geq}(t_1, t_2)^2 & AG_{\uparrow\uparrow}^{\geq}(t_1, t_2)^2 G_{\uparrow\downarrow}^{\geq}(t_1, t_2) + \xi^2 G_{\uparrow\downarrow}^{\geq}(t_1, t_2)^3 \\ AG_{\uparrow\uparrow}^{\geq}(t_1, t_2)^2 G_{\uparrow\downarrow}^{\geq}(t_1, t_2) + \xi^2 G_{\uparrow\downarrow}^{\geq}(t_1, t_2)^3 & -\xi^2 G_{\uparrow\uparrow}^{\geq}(t_1, t_2)^3 + AG_{\uparrow\uparrow}^{\geq}(t_1, t_2)G_{\uparrow\downarrow}^{\geq}(t_1, t_2)^2 \end{pmatrix}, \quad (33)$$

Therefore, following the same steps, the linearization of the Schwinger-Dyson equation  $G^K = G^R \circ \Sigma^K \circ G^A$  leads to

$$\begin{aligned} \delta G_{\uparrow\downarrow}^K(t_1, t_1) &= \left[ G_{\uparrow\uparrow}^{R, \beta_f} \circ \delta \Sigma_{\uparrow\downarrow}^K \circ G_{\uparrow\uparrow}^{A, \beta_f} \right] (t_1, t_1), \\ \delta \Sigma_{\uparrow\downarrow}^K(t_1, t_2) &= \frac{1}{4}J^2 A \delta(t_1 - t_2) \left( G_{\uparrow\uparrow}^{>, \beta_f}(t_1, t_1)^2 + G_{\uparrow\uparrow}^{<, \beta_f}(t_1, t_1)^2 \right) \delta G_{\uparrow\downarrow}^K(t_1, t_1). \end{aligned} \quad (34)$$

To form close equation groups, we set the time argument of the first equation to be  $(t_1, t_1)$ , and then we study the equal time perturbation of the Green's function  $\delta G_{\uparrow\downarrow}^K(t, t)$ .

Using the high-temperature solution, we get

$$\begin{aligned} \delta G_{\uparrow\downarrow}(t_1, t_1) &= \int dt_2 G_{\uparrow\uparrow}^R(t_1, t_2) \left( -\frac{1}{8}J^2 A e^{-|t_2 - t_1|\Gamma} \delta G_{\uparrow\downarrow}(t_2, t_2) \right) G_{\uparrow\downarrow}^A(t_2, t_1) \\ &= -\frac{1}{8}J^2 A \int dt_2 e^{-\frac{\Gamma}{2}(t_1 - t_2)} \Theta(t_1 - t_2) \delta G_{\uparrow\downarrow}(t_2, t_2) e^{\frac{\Gamma}{2}(t_2 - t_1)} \Theta(-t_2 + t_1). \\ &= -\frac{1}{8}J^2 A \int dt_2 e^{-\Gamma(t_1 - t_2)} \Theta(t_1 - t_2) \delta G_{\uparrow\downarrow}(t_2, t_2). \end{aligned} \quad (35)$$

Multiply  $e^{\Gamma t_1}$  and take  $\partial_{t_1}$  on the Eq. (35), which gives

$$\partial_{t_1} [e^{\Gamma t_1} \delta G_{\uparrow\downarrow}(t_1, t_1)] = -\frac{1}{8}J^2 A \int dt_2 e^{\Gamma t_2} \delta(t_1 - t_2) \delta G_{\uparrow\downarrow}(t_2, t_2). \quad (36)$$

Finally leads to

$$(\partial_t + \Gamma) \delta G_{\uparrow\downarrow}^K(t, t) = -\frac{AJ}{8} \delta G_{\uparrow\downarrow}^K(t, t). \quad (37)$$

Solving this differential equation leads to  $\delta G_{\uparrow\downarrow}^K(t, t) \sim m(t) \sim e^{-(\Gamma + AJ/8)t}$  with a simple exponential decay.



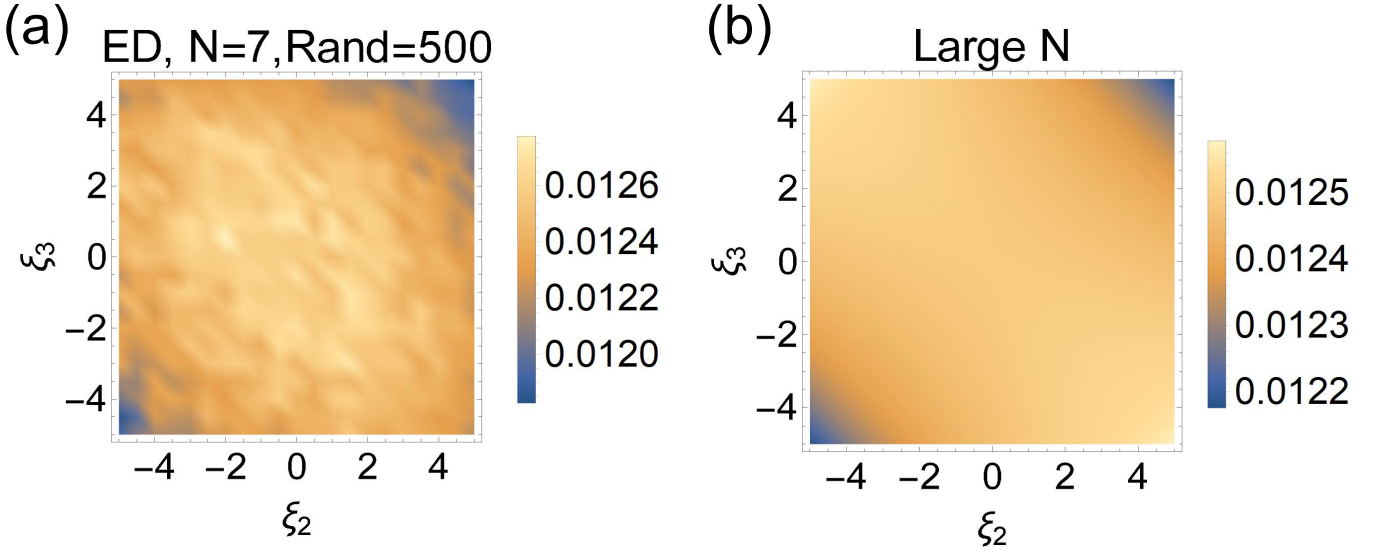

FIG. 4. (a) The susceptibility of the exact diagonalization numerics. We choose site number  $N = 7$ , and random realizations to be 500. (b) The susceptibility of the large- $N$  numerics. In both cases, to obtain the susceptibility, we choose the equilibrium thermal state with temperature  $T/J = 10.0$ , and external magnetic field with  $h/J = 0.05$  in  $x$  direction. We take the region of anisotropic parameter  $\xi_2, \xi_3$  to be  $[-5, 5]$ , and the discretization step is  $\Delta\xi = 0.5$ .

## VII. SUSCEPTIBILITY IN THERMAL EQUILIBRIUM

As we discussed in the main text, we calculate the equilibrium susceptibility. We take a small external magnetic field in the  $x$  direction in the equilibrium thermal state. The finite difference susceptibility is defined as  $\chi = \langle \hat{S}_x \rangle_h / h$ , where  $\langle \hat{S}_x \rangle_h$  means the thermal average in the external magnetic field  $h$ . First, we find the exact diagonalization and large- $N$  Kadanoff-Baym results in fig. 4 agree well with each other. Second, equilibrium susceptibility in fig. 4 is highly in contrast with the criterion for the relaxation dynamics  $A$  in fig. 3. There is no appreciable distinction between  $A > 0$  and  $A < 0$  region correspondingly in the plot of the equilibrium. Hence, it reveals the significance of our dynamical framework.
